# Supplementary material for: Comparing Overlapping Data Distributions Using Visualization
Source: arXiv:2309.12667 source file (2023-09-22)
Supplement: Supplementary file 1 [file appendix.tex]

\clearpage
\appendix
\newpage
\pagenumbering{arabic}

\onecolumn
\setcounter{page}{1}
\setcounter{section}{0}
    
\begin{center}
\huge{\textsf{\papertitle}}

\Large\textsf{Supplementary Materials}
\end{center}

\section{Study Instructions}

[...]

% \section{Stimulus Datasets}

% We have attached a CSV file containing the 12 datasets used for the trials: 2 spreads $S \times $ 2 dataset sizes $D \times$ 3 repetitions.

\section{Anonymized Performance Data}

We have attached the unfiltered but anonymized performance data for all participants. 
In other words, the provided dataset has \textbf{not} been filtered based on the attention (training) trials, completion time, mean difference, or standard deviation.
